# Supplementary material for: Formally Exact Simulations of Mesoscale Exciton Diffusion in a Photosynthetic Aggregate
Source: arXiv:2301.04537 source file (2023-01-11)
Supplement: Supplementary file 1 [file LH2_SI.pdf]

# Supporting Information: Formally Exact Simulations of Mesoscale Exciton Diffusion in a Photosynthetic Aggregate

Leonel Varvelo,[1, a)] Jacob K. Lynd,[1, a)] Brian Citty,[1] Oliver Kühn,[2] and Doran I. G. B. Raccah[1]
[1)]*Department of Chemistry, Southern Methodist University, PO Box 750314, Dallas, TX, USA*
[2)]*Institute of Physics, University of Rostock, Albert-Einstein-Str. 23-24, 18059 Rostock, Germany*

(Dated: 11 January 2023)

## S1. LH2 HAMILTONIAN

Table S1 shows the LH2 B850 Hamiltonian used for all calculations presented here.[1,2]

## S2. MATSUBARA DECOMPOSITION

The bath correlation function is described by a Drude-Lorentz spectral density $J_n(\omega)$ (eq. 9, main text), and is decomposed into a collection of exponential contributions

$$C_n(t) = \sum_{j_n} g_{j_n} e^{-\gamma_{j_n} t/\hbar}. \tag{S1}$$

The specific values of $g_{j_n}$ and $\gamma_{j_n}$ are given by the Matsubara decomposition of the Drude-Lorentz spectral density:

$$g_{0_n} = 2\lambda_n \beta^{-1}\left(1 + \sum_{j=1}^{k_{Mats}} \frac{\gamma_{0_n}^2}{\gamma_{0_n}^2 - \gamma_{j_n}^2}\right) - i\lambda_n\gamma_{0_n} \tag{S2}$$

for the "high-temperature" mode, and

$$g_{j_n} = \frac{2i}{\beta} J_n(i\gamma_{j_n}), \quad \gamma_{j_n} = \frac{2\pi j}{\beta} \tag{S3}$$

for Matsubara modes $j \neq 0$, where $k_{Mats}$ is the number of Matsubara modes included. To ensure that $C(-t) = C^*(t)$, we also include one other mode in each correlation function with a prefactor

$$g_{Mark_n} = i\lambda_n\gamma_{0_n} \tag{S4}$$

and a decay timescale that matches the fastest-decaying Matsubara mode.

## S3. ADAPTIVE HIERARCHY OF PURE STATES (ADHOPS)

In a HOPS calculation, the physical wave function localizes in the presence of a thermal bath.[3] The localization in the physical wave function induces localization in the basis of auxiliary wave functions. With a localized physical wave function and localized hierarchy an adaptive solution (adHOPS) to the HOPS equation of motion becomes advantageous.[3] A reduced basis set consisting of a direct sum of a restricted set of essential auxiliaries ($\mathbb{A}_t$) and states ($\mathbb{S}_t$) is created every $u_t$ femtoseconds (the 'update time') during the time-evolution of an adHOPS trajectory. The user-defined truncation parameter ($\delta$) represents a bound on the derivative error in the evolution of the full state (physical and auxiliary wave functions) over one timestep. The derivative error is defined in terms of Euclidean distance between the true derivative vector and the effective derivative vector constructed using the adaptive basis. $\delta$ can be further decomposed into two parts: the bound of the error associated with neglecting system states ($\delta_S$) and the bound on the error associated with neglecting auxiliary wave functions ($\delta_A$) such that $\delta^2 = \delta_S^2 + \delta_A^2$. The reduced basis constructed does not impose locality on the physical wave function: rather, it takes advantage of any locality that is already present in the calculation. If the full basis is needed to satisfy $\delta$, adHOPS reverts back to a HOPS calculation. In summary, the adaptive HOPS algorithm is a formally exact method of calculating open quantum system dynamics that achieves size-invariant scaling when the size of a molecular aggregate greatly exceeds the delocalization extent of the exciton.

### A. Convergence Parameters

The accuracy of an adHOPS calculation is controlled by a set of parameters, referred to generically as 'convergence parameters.'

*a. Hierarchy Depth ($k_{max}$):* The maximum allowed sum of the auxiliary wave function index vector values ($\sum_n \vec{k}[n] \leq k_{max}$), also known as the triangular truncation depth.

*b. Hierarchy Adaptive Error Limit ($\delta_A$):* The maximum allowable derivative error stemming from neglecting hierarchy elements (i.e., auxiliary wave functions) when updating the basis. If this parameter is set to 0, the basis of auxiliary wave functions will always be the complete set defined by the triangular truncation condition.

*c. State Adaptive Error Limit ($\delta_S$):* The maximum allowable derivative error stemming from neglecting state basis elements (i.e., pigments corresponding to Hamiltonian/wave function indices) when updating the basis. If this parameter is set to 0, the state basis is the full state basis of the Hamilto-

---

[a)]Co-first author: These authors contributed equally and authorship order was determined by a coin-toss. All authors agree that these authors may list themselves in either order for their CV/Resume and other purposes.

| A BCL 301 | B BCL 302 | C BCL 303 | D BCL 304 | E BCL 305 | F BCL 306 | A1 BCL 301 | B1 BCL 302 | C1 BCL 303 | D1 BCL 304 | E1 BCL 305 | F1 BCL 306 | A2 BCL 301 | B2 BCL 302 | C2 BCL 303 | D2 BCL 304 | E2 BCL 305 | F2 BCL 306 |
|---|---|---|---|---|---|---|---|---|---|---|---|---|---|---|---|---|---|
| 12,700 | 307 | −50.9 | 13 | −6.08 | 2.83 | −1.8 | 1.08 | −0.93 | 0.71 | −0.93 | 0.98 | −1.8 | 2.6 | −6.08 | 13.2 | −50.9 | 237 |
| 307 | 12,100 | 237 | −35 | 13.2 | −4.22 | 2.6 | −1.11 | 0.98 | −0.47 | 0.71 | −0.47 | 1.08 | −1.11 | 2.83 | −4.22 | 13 | −35 |
| −50.9 | 237 | 12,700 | 307 | −50.9 | 13 | −6.08 | 2.83 | −1.8 | 1.08 | −0.93 | 0.71 | −0.93 | 0.98 | −1.8 | 2.6 | −6.08 | 13.2 |
| 13 | −35 | 307 | 12,100 | 237 | −35 | 13.2 | −4.22 | 2.6 | −1.11 | 0.98 | −0.47 | 0.71 | −0.47 | 1.08 | −1.11 | 2.83 | −4.22 |
| −6.08 | 13.2 | −50.9 | 237 | 12,700 | 307 | −50.9 | 13 | −6.08 | 2.83 | −1.8 | 1.08 | −0.93 | 0.71 | −0.93 | 0.98 | −1.8 | 2.6 |
| 2.83 | −4.22 | 13 | −35 | 307 | 12,100 | 237 | −35 | 13.2 | −4.22 | 2.6 | −1.11 | 0.98 | −0.47 | 0.71 | −0.47 | 1.08 | −1.11 |
| −1.8 | 2.6 | −6.08 | 13.2 | −50.9 | 237 | 12,700 | 307 | −50.9 | 13 | −6.08 | 2.83 | −1.8 | 1.08 | −0.93 | 0.71 | −0.93 | 0.98 |
| 1.08 | −1.11 | 2.83 | −4.22 | 13 | −35 | 307 | 12,100 | 237 | −35 | 13.2 | −4.22 | 2.6 | −1.11 | 0.98 | −0.47 | 0.71 | −0.47 |
| −0.93 | 0.98 | −1.8 | 2.6 | −6.08 | 13.2 | −50.9 | 237 | 12,700 | 307 | −50.9 | 13 | −6.08 | 2.83 | −1.8 | 1.08 | −0.93 | 0.71 |
| 0.71 | −0.47 | 1.08 | −1.11 | 2.83 | −4.22 | 13 | −35 | 307 | 12,100 | 237 | −35 | 13.2 | −4.22 | 2.6 | −1.11 | 0.98 | −0.47 |
| −0.93 | 0.71 | −0.93 | 0.98 | −1.8 | 2.6 | −6.08 | 13.2 | −50.9 | 237 | 12,700 | 307 | −50.9 | 13 | −6.08 | 2.83 | −1.8 | 1.08 |
| 0.98 | −0.47 | 0.71 | −0.47 | 1.08 | −1.11 | 2.83 | −4.22 | 13 | −35 | 307 | 12,100 | 237 | −35 | 13.2 | −4.22 | 2.6 | −1.11 |
| −1.8 | 1.08 | −0.93 | 0.71 | −0.93 | 0.98 | −1.8 | 2.6 | −6.08 | 13.2 | −50.9 | 237 | 12,700 | 307 | −50.9 | 13 | −6.08 | 2.83 |
| 2.6 | −1.11 | 0.98 | −0.47 | 0.71 | −0.47 | 1.08 | −1.11 | 2.83 | −4.22 | 13 | −35 | 307 | 12,100 | 237 | −35 | 13.2 | −4.22 |
| −6.08 | 2.83 | −1.8 | 1.08 | −0.93 | 0.71 | −0.93 | 0.98 | −1.8 | 2.6 | −6.08 | 13.2 | −50.9 | 237 | 12,700 | 307 | −50.9 | 13 |
| 13.2 | −4.22 | 2.6 | −1.11 | 0.98 | −0.47 | 0.71 | −0.47 | 1.08 | −1.11 | 2.83 | −4.22 | 13 | −35 | 307 | 12,100 | 237 | −35 |
| −50.9 | 13 | −6.08 | 2.83 | −1.8 | 1.08 | −0.93 | 0.71 | −0.93 | 0.98 | −1.8 | 2.6 | −6.08 | 13.2 | −50.9 | 237 | 12,700 | 307 |
| 237 | −35 | 13.2 | −4.22 | 2.6 | −1.11 | 0.98 | −0.47 | 0.71 | −0.47 | 1.08 | −1.11 | 2.83 | −4.22 | 13 | −35 | 307 | 12,100 |

TABLE S1. The Hamiltonian for the B850 ring.[1,2]

nian.

*d. Timestep ($dt$):* The timestep of numerical integration of the equation of motion.

*e. Matsubara Modes ($k_{Mats}$):* The number of Matsubara modes included in the correlation function. As this parameter goes to infinity, the exponential form of the correlation function approaches the analytic solution of Eq. (2) of the main text.

*f. Update Time ($u_t$)* The computational bottleneck in adaptive HOPS calculations is the process of updating the state and auxiliary bases at each time point. As a result, it is possible to significantly reduce the calculation time by updating the basis only every $u_t$ fs of the simulation (with those time points designated as 'update steps').

## B. Computational Details

Schema S1(a) shows the adHOPS algorithm.

### 1. *time-evolution*

The adHOPS algorithm consists of repeated time integration of the HOPS equation given by eq. (5), broken up by updates to the adaptive basis. During time-evolution, a sparse super-operator $\hat{K}_t$ is defined such that $\hat{K}_t|\phi\rangle_t = \partial_t|\phi\rangle_t$, where $|\phi\rangle_t$ is the vector defining the full state of the system and bath, including all auxiliary wave functions in the current basis, at time $t$. With this operator defined, we use fourth-order Runge-Kutta integration to calculate $|\phi\rangle_{t+dt} = |\phi\rangle_t + \int_t^{t+dt} \hat{K}_t|\phi\rangle_\tau d\tau$. At this point, quantities $\langle\hat{L}_n\rangle_{t+dt}$, $\xi_{n,t+dt}$, and $\Gamma_{t+dt}$ are calculated based on eqs. (6-8) for use in the calculation of $\hat{K}_{t+dt}$.

### 2. *Basis Update Steps*

When a time step is designated as an update step, adHOPS constructs a new basis set immediately after time-evolution. This process is detailed in Schema S1(b).We can break down the basis construction into two steps: constructing the new auxiliary basis ($\mathbb{A}_{t+dt}$), introducing derivative error no greater than $\delta_A$, and constructing the new state basis ($\mathbb{S}_{t+dt}$), introducing derivative error no greater than $\delta_S$. When the direct sum basis is constructed, the order in which each basis is treated can influence the reduced basis. In our current adHOPS implementation we construct the new auxiliary basis before the new state basis.

The first step in constructing a new auxiliary basis is to calculate the derivative error associated with the exclusion of "stable" auxiliaries (elements in the current basis $\mathbb{A}_t$). The derivative error associated with removing a given auxiliary wave function is given by the $L_2$ norm of the resulting change in the derivative vector. The adaptive algorithm sorts this error from lowest to highest, and selects a cutoff point where the sum of the error is the maximum allowable error $E_A$ (that is, the maximum possible error for which $E_A \leq \delta_A/2$). Finally,

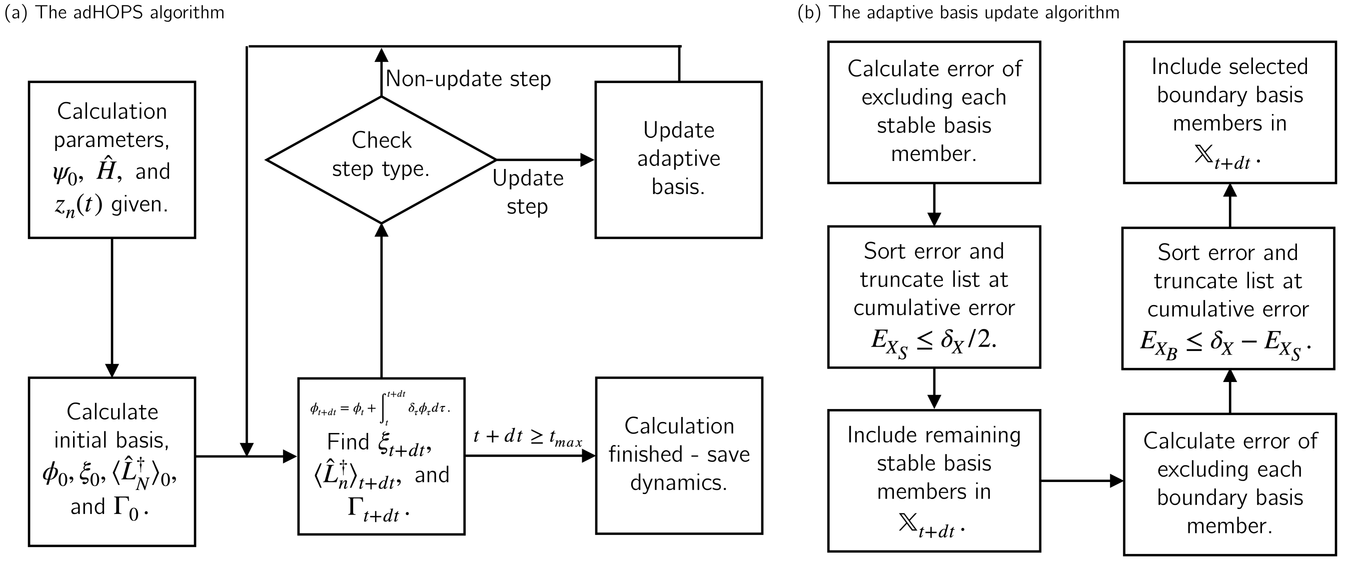


Scheme S1. The adHOPS algorithm. (a) The overarching algorithm that an adaptive HOPS simulation follows. (b) The algorithm that updates the adaptive HOPS basis during update steps. "Stable basis" refers to the basis from the previous time step, while "boundary basis" refers to the terms that would be populated by main text eq. (5)

stable basis members beyond the cutoff point are included in $\mathbb{A}_{t+dt}$.

Next, the algorithm considers the derivative error associated with continuing to exclude the "boundary" auxiliaries (basis elements that are not included in the current basis, but which would be populated by eq. (5)). The algorithm sorts these elements from lowest to highest associated error, then includes elements in the basis up to a cutoff point such that the error associated with continuing to exclude the remaining boundary elements is the maximum allowable that is bounded by $\delta_A - E_A$.

Finally, this process is repeated for the state basis, with $\delta_S$ replacing $\delta_A$. The derivative error associated with excluding a state basis element is given by the $L_2$ norm over the hierarchy basis $\mathbb{A}_t$: to avoid double-counting error associated with the exclusion of stable hierarchy elements, the stable hierarchy elements that have been filtered out during the construction of $\mathbb{A}_{t+dt}$ are ignored during the calculation of derivative error for excluding state basis members.

### 3. *Markovian Filter*

When a correlation function mode $C_{j_n}(t) = g_{j_n} e^{-\gamma_{j_n} t/\hbar}$ decays on a sufficiently fast timescale, the auxiliary wave functions at depth one in the hierarchy fully describe the overall dynamics. In order to reduce the size of the basis without sacrificing accuracy, we apply a Markovian filter to the appropriate modes: with this filter, the only auxiliary wave functions with non-zero indices along the Markovian modes are the auxiliaries at depth one in the hierarchy ($\sum_n \vec{k}[n] = 1$). This Markovian filter is highly efficient when used in conjunction with adaptivity: since there are no higher-lying auxiliary wave functions that the Markovian auxiliary wave function may influence, only its contributions to the physical wave function need be considered. Thus, the Markovian filter speeds up both adaptive basis construction and time-evolution. We use the Markovian filter on all modes other than the high-temperature mode.

### 4. *Early-Time Inchworming*

At early time, the adaptive bases are comparatively small and evolve rapidly in time. To construct the initial adaptive basis, the earliest ten time steps are calculated with an inchworming integrator that recalculates the basis $s_i$ times (the 'inchworm step') after every time-evolution. This ensures that the adaptive basis at early times expands rapidly to capture the initial dynamics. For all simulations referenced in this paper, we set $s_i$ to 2.

### 5. *Sampling Noise Trajectories*

We construct correlated complex-valued noise trajectories ($z^*_{n,t}$) associated with a single pigment ($n$) that satisfies the conditions $\mathbb{E}[z_{n,t}] = 0$, $\mathbb{E}[z_{n,t} z_{n,s}] = 0$, and $\mathbb{E}[z^*_{n,t} z_{n,s}] = C_n(t - s)$ using the circulant embedding method.[4] We briefly summarize the algorithm below.

- **Step 1:** We sample the correlation function $s_{n,m} = C_n(t_m)$ at $N_t$ evenly spaced points $t_m = m\frac{T_{\text{noise}}}{N_t}$ for $m =$

$0,\ldots,N_t-1$, where $T_{\text{noise}}$ is the length of the noise trajectory.

- **Step 2:** We rotate the samples such that at the last time point, the sample is real $s_{n,m} = \tilde{C}_n(t_m) = C_n(t_m)e^{-i2\pi\nu t_m}$, where $\nu = \text{phase}(C_n(t_{N_t-1}))/(t_{N_t-1}\pi)$.
- **Step 3:** We extend the vector to size $2N-2$ by defining $s_{n,2N_t-2-m} = s^*_{n,m}$ for $m = 1,\ldots,N_t-2$. The rotation $(e^{-i2\pi\nu t_m})$ allows us to reduce the size of this embedding from $2N_t-1$ to $2N_t-2$, equivalent to the case for real noise.
- **Step 4:** We calculate $S_{n,k}$ as the Fourier transform of the vector $\boldsymbol{s}_n$ (known as the 'circulant embedding'). $S_{n,k}$ are the (real) eigenvalues of the covariance matrix $(\tilde{C}_n)$.
- **Step 5:** Negative eigenvalues (i.e., $S_{n,k} < 0$) are set to 0.
- **Step 6:** We define the sequence $W_{n,k} = (Z_{n,2k} + iZ_{n,2k+1})\sqrt{S_{n,k}/2}$ for $k = 0,\ldots,N_t$, where $Z_{n,2k}$ and $Z_{n,2k+1}$ are Fourier transformed vectors of uncorrelated noise sampled from a complex normal distribution with mean 0 and variance 2.
- **Step 7:** We find sampled process $\tilde{z}_{n,t}$ via the inverse Fourier transform of $W_k$, sampled at time $t_m$ for $m = 0,\ldots,N_t-1$.
- **Step 8:** Finally, we rotate the sampled process back to back to the original phase $z_{n,t} = \tilde{z}_{n,t}e^{-i2\pi\nu t}$.

## S4. DETERMINATION OF CONVERGENCE PARAMETERS

To ensure the adHOPS dynamics are converged, we measure the population error introduced by reducing the stringency of convergence parameters. Population error is given by the L1 norm of the difference between the population vectors of two ensemble averages run with different convergence parameters:

$$\sum_t \frac{\|\vec{P}(t) - \vec{P}_{ref}(t)\|_1}{N_t} \tag{S5}$$

where $\vec{P}(t)$is the population vector of the test ensemble, $\vec{P}_{ref}(t)$ is the population vector of some reference ensemble, and $N_t$ is the number of time points. These population vectors may be given in any basis and with any coarse-graining (e.g., they may measure the population of individual pigments or individual B850 rings).

We converge a parameter by varying its value and measuring error with respect to a parameter-specific reference ensemble (we refer to this as a 'convergence scan' of a parameter). The reference ensemble's convergence parameters are either intentionally over-converged or verified by other convergence scans. We consider a parameter converged if it introduces a population error of 0.02 or less with respect to the reference ensemble (this is represented in Figs. S1-S5 by a gray shaded region). To ensure that error stems from only the shifted parameter, we match the noise trajectories and static disorder distributions of the tested and reference ensemble.

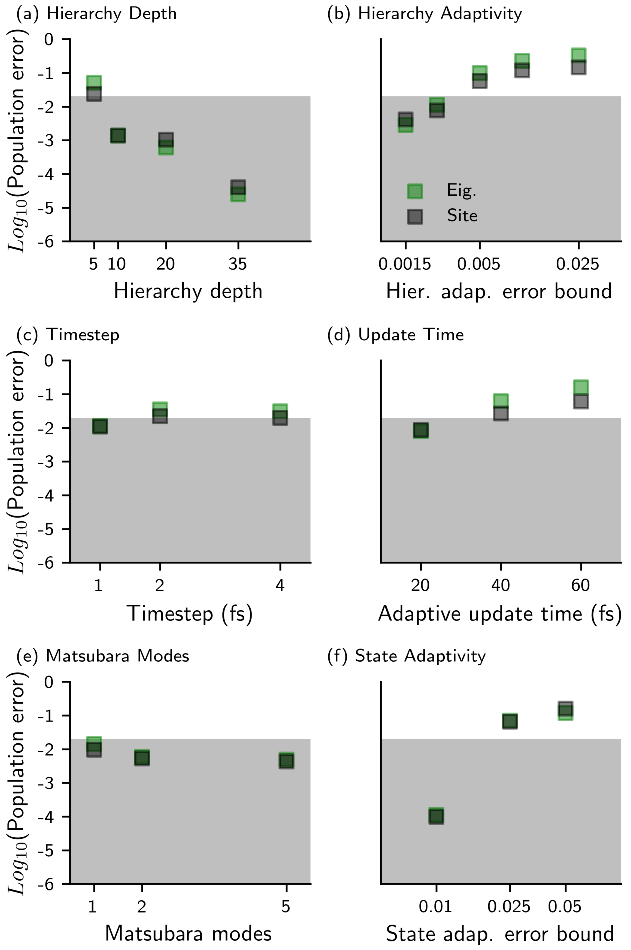


FIG. S1. Parameter convergence of the LH2 monomer in terms of site (black) and eigenstate (green) populations. In all cases, $\sigma = 68\ \text{cm}^{-1}$ for site energy static disorder. The gray shaded region represents the convergence threshold where mean population error is 0.02 or less. Population error with respect to (a) $k_{max}$, compared to a reference $k_{max}$ of 50, (b) $\delta_A$, compared to a reference $\delta_A$ of 0.0005, (c) $dt$, compared to a reference $dt$ of 0.5 fs, (d) $u_t$, compared to a reference $u_t$ of 10 fs, (e) $k_{Mats}$, compared to a reference $k_{Mats}$ of 10, and (f) $\delta_S$, compared to a reference of the full state basis. Full set of convergence parameters given in Table S6.

In all cases, convergence scans were run without angular static disorder. In addition, due to a translation error, we employed a site energy static disorder with a standard deviation $\sigma = 68\ \text{cm}^{-1}$. This change from the main text value of $\sigma = 160\ \text{cm}^{-1}$ does not influence the convergence results.

### A. Monomer Convergence Parameters

In Fig. S1, we examine population error in terms of both monomer eigenstate and individual Bchl ('site') populations over 400 fs. Both populations have equivalent convergence (within statistical error) and exhibit monotonic error decay as each parameter is made more stringent. The sudden decay of population error with respect to $\delta_S$ indicates that the vast majority of states are occupied in the monomer. The slight benefits to basis size by incorporating a state adaptive error bound are thus outweighed by the computational time spent constructed an adaptive state basis for small B850 complexes. Furthermore, while a hierarchy depth of 10 appears to be over-converged, the cost of increasing the hierarchy depth when the auxiliary basis is constructed adaptively is minimal. Therefore, going forward, we assume that $k_{max} = 10$ is converged for B850 complexes.

### B. Dimer Convergence Parameters

In Figs. S2-S4, we examine population error in terms of the populations of the individual eigenstates of each B850 ring, as well as the populations of the full B850 rings. We note that the error of the eigenstate populations must be the upper bound on the error of the ring populations.

#### 1. Dimer (R = 6.5 nm)

In Fig. S2, we demonstrate the convergence of adHOPS simulations of the $R = 6.5$ nm dimer over 400 fs. The dynamics of the exciton populations summed over B850 rings (i.e., ring populations) converge at far less stringent parameters than the dynamics of the eigenstate populations. We note that this indicates that characterizing convergence via the simplest observable that captures the dynamics of interest (in this case, the populations of the B850 rings representing the dimeric dynamics that we extract a rate from) can significantly reduce the computational expense of adHOPS simulations.

#### 2. Dimer (R = 7.5 nm)

In Fig. S3, we demonstrate the convergence of adHOPS simulations of the $R = 7.5$ nm dimer over 3 ps in terms of the population of the full B850 rings. Rather than scan for convergence with respect to Matsubara modes, we use $k_{Mats} \geq 5$ in all $R = 7.5$ nm simulations to ensure convergence.

#### 3. Dimer (R = 8.5 nm)

In Fig. S4, we demonstrate the convergence of adHOPS simulations of the $R = 8.5$ nm dimer over 5 ps in terms of the population of the full B850 rings. Rather than scan for convergence with respect to Matsubara modes and timestep, we use $k_{Mats} \geq 5$ and $dt \leq 0.5$ fs in all $R = 8.5$ nm simulations to ensure convergence.

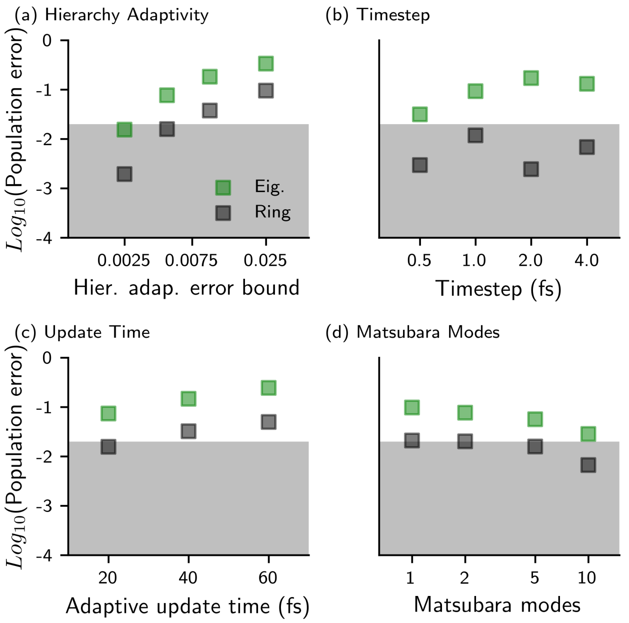


FIG. S2. Parameter convergence of the $R = 6.5$ nm B850 dimer in terms of eigenstate (green) and ring (black) populations. In all cases, angular static disorder was neglected and $\sigma = 68\ \text{cm}^{-1}$ for site energy static disorder. The gray shaded region represents the convergence threshold where mean population error is 0.02 or less. Population error with respect to (a) $\delta_A$, compared to a reference $\delta_A$ of 0.001, (b) $dt$, compared to a reference $dt$ of 0.5 fs, (c) $u_t$, compared to a reference $u_t$ of 2.0 fs, and (d) $k_{Mats}$, compared to a reference $k_{Mats}$ of 20. Full set of convergence parameters given in Table S6.

### C. Heptamer Convergence Parameters

In Fig. S5a-e, we demonstrate the convergence of a $R = 6.5$ nm B850 heptamer in terms of ring populations and the populations of the center donor and set of six B850 rings forming the first shell of acceptors. We note that the converged parameters are the same values as in the $R = 6.5$ nm dimer, excepting $\delta_S$. As such, we present the convergence of this heptamer to demonstrate that the only parameter necessary to converge for the 37-mer is $\delta_S$.

### D. 37-mer Convergence Parameters

In Fig. S5f, we demonstrate the convergence of the $R = 6.5$ nm 37-mer B850 super-complex in terms of ring populations and the populations of the concentric hexagonal shells of rings making up the complex with respect to $\delta_S$. The converged values of $k_{max}$, $\delta_A$, $dt$, $k_{mats}$, and $u_t$ should be the same as those of the heptamer.

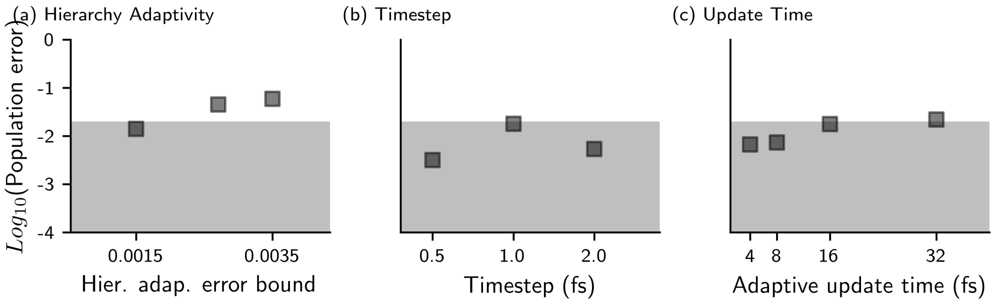


FIG. S3. Parameter convergence of the $R = 7.5$ nm B850 dimer in terms of ring populations. In all cases, angular static disorder was neglected and $\sigma = 68$ $\mathrm{cm}^{-1}$ for site energy static disorder. The gray shaded region represents the convergence threshold where mean population error is 0.02 or less. Population error with respect to (a) $\delta_A$, compared to a reference $\delta_A$ of 0.001, (b) $dt$, compared to a reference $dt$ of 0.25 fs, and (c) $u_t$, compared to a reference $u_t$ of 2.0 fs. Full set of convergence parameters given in Table S6.

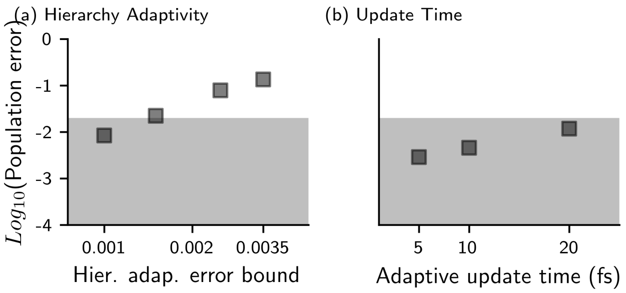


FIG. S4. Parameter convergence of the $R = 8.5$ nm B850 dimer in terms of ring populations. In all cases, angular static disorder was neglected and $\sigma = 68$ $\mathrm{cm}^{-1}$ for site energy static disorder. The gray shaded region represents the convergence threshold where mean population error is 0.02 or less. Population error with respect to (a) $\delta_A$, compared to a reference $\delta_A$ of 0.0005, and (b) $u_t$, compared to a reference $u_t$ of 2.0 fs. Full set of convergence parameters given in Table S6.

## S5. SAMPLING STATIC DISORDER

We employ two types of static disorder in our calculations: site energy static disorder and angular static disorder. Site energy static disorder accounts for random fluctuations in site energies stemming from movements of the protein structure on timescales longer than the simulation, and is represented by shifting the diagonal entries of the system Hamiltonian $H_S$. These shifts in site energies are given by a real-valued Gaussian distribution of width $\sigma$ centered on 0. Angular static disorder accounts for the randomness of LH2 orientations inside of a membrane, and is represented by rotating the $n^{\text{th}}$ LH2 in a given aggregate by some angle $\theta_n$ about its nine-fold symmetric axis normal to the membrane. The values of $\theta_n$ were randomly selected from a uniform distribution.

When introducing static disorder into the calculations, we randomly sample a set of site energy displacements ($\mathbf{E} = [\Delta E_1, \Delta E_2, ..., \Delta E_{N_{\text{chl}}}]$), a set of angular orientations for each LH2 ($\mathbf{\Theta} = [\theta_1, \theta_2, ..., \theta_{N_{\text{B850}}}]$), and a set of noise trajectories associated with each pigment ($\mathbf{z}^* = [z^*_{1,t}.z^*_{2,t}, ..., z^*_{N_{\text{chl}},t}]$ before each calculation. This can be interpreted as converting the Monte Carlo sampling over the space of noise trajectories ($\mathbf{z}^*$) introduced by the HOPS derivation into a simultaneous Monte Carlo sampling over the combined space of ($\mathbf{E}, \mathbf{\Theta}, \mathbf{z}^*$). Because each of the spaces being sampled are independent, they can be simultaneously Monte Carlo sampled without losing efficiency. This is one of the advantages to stochastic wave function approaches.

## S6. EXTRACTING DIMER RATES

The rates of exciton transport in B850 dimers ($\kappa_{dimer}$) are constructed from an exponential fit to the long-time population dynamics. Figure S6 compares the adHOPS dynamics (solid lines) with a single exponential fit starting at 600 fs (dashed lines, $\kappa_{dimer} = 0.44 \pm 0.04$ $\mathrm{ps}^{-1}$) for the dimer with inter-ring distance $R = 6.5$ nm. The starting time for the exponential fit (600 fs) was selected to ensure that the subsequent population dynamics are well described by a single rate process. The dimer rates at inter-ring distances of 7.5 and 8.5 nm are not sensitive to the choice of initial time, though we still used a starting time of 600 fs for the kinetic fitting to ensure consistency.

## S7. STATIC DISORDER AND $L_d$

To investigate the roles of static disorder in the reported excitation diffusion lengths, we compared calculations with all combinations of site energy and angular static disorder. We found the corresponding rates of population transport $\kappa_{dimer}$ by fitting the adHOPS population dynamics of the B850 rings starting from 600 fs to a single exponential, as outlined in section S6. In each case, the ensemble consisted of $N_{traj} = 10^4$ trajectories where our realizations of energetic and angular disorder, along with the noise trajectories, are matched between ensembles (see Sec. S5 for details). The squared-diffusion rate $D$ and length $L_d$ in an infinite hexagonally-

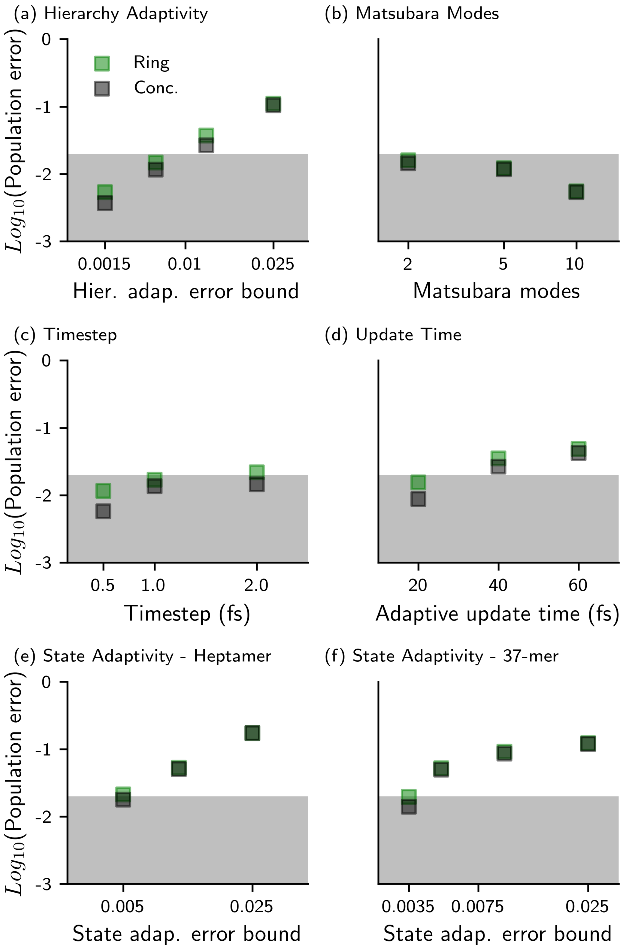


FIG. S5. Parameter convergence of the LH2 heptamer and 37-mer in terms of B850 ring (green) and concentric shell (black) populations. In all cases, angular static disorder was neglected and $\sigma = 68 \text{ cm}^{-1}$ for site energy static disorder. The gray shaded region represents the convergence threshold where mean population error is 0.02 or less. Population error of the heptamer with respect to (a) $\delta_A$, compared to a reference $\delta_A$ of 0.001, (b) $k_{Mats}$, compared to a reference $k_{Mats}$ of 20, (c) $dt$, compared to a reference $dt$ of 0.25 fs, (d) $u_t$, compared to a reference $u_t$ of 8.0 fs, and (e) $\delta_S$, compared to a reference of the full state basis. (f) Population error of the 37-mer with respect to $\delta_S$, compared to a reference $\delta_S$ of 0.0025. Full set of convergence parameters given in Table S6.

packed aggregate were given by

$$L_d^2 = D\tau = 6\kappa_{dimer}R^2\tau \tag{S6}$$

where the exciton lifetime $\tau$ was assumed to be 1 ns[5] (see section S9 for details).

The effects of static disorder on diffusion of the excitation distribution, reported in Table S2, are almost entirely attributable to site energy static disorder. While the presence of angular static disorder leads $L_d$ to decrease by 10 nm, the presence of site energy static disorder is responsible for a far more significant decrease of 100 nm. Although sufficient synthetic ingenuity might allow for precise control of angular organization within an LH2 aggregate, similar control of the site energy distributions seems implausible. As such, extending the $L_d$ of LH2 hybrid materials by suppressing static disorder is unlikely to be a fruitful endeavor.

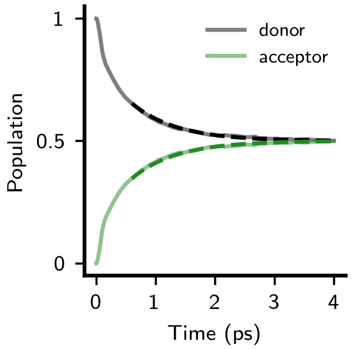


FIG. S6. B850 dimer adHOPS population dynamics (solid line) and exponential fit (dashed line) starting from 600 fs. The exponential is fit to a single rate $\kappa_{dimer}$. The dynamics pictured are for a dimer with $R = 6.5$ nm, $\sigma = 160 \text{ cm}^{-1}$ for site energy static disorder, and angular static disorder given by randomly orienting both B850 rings in each trajectory. This adHOPS calculation and corresponding rate are also referenced in Fig. S7b in the case with $R = 6.5$ nm and all couplings allowed. Full set of convergence parameters given in Table S6.

| Static disorder type | $\kappa_{dimer}$ (ps$^{-1}$) | D (nm$^2$/ps) | $L_d$ (nm) |
|---|---|---|---|
| Site energy and angular | 0.44 ±0.040 | 110 ±10. | 330 ±15 |
| Site energy only | 0.47 ±0.048 | 120 ±12 | 340 ±18 |
| Angular only | 0.72 ±0.107 | 180 ±27 | 430 ±33 |
| None | 0.77 ±0.0108 | 190 ±27 | 440 ±30. |

TABLE S2. The kinetically-derived exciton transfer rate $\kappa_{dimer}$, excitation diffusion rate $D$, and diffusion length $L_d$ for B850 aggregates in a hexagonally-packed lattice with various combinations of static disorder. The site energy static disorder is given by a Gaussian distribution with $\sigma = 160 \text{ cm}^{-1}$, and the angular static disorder is given by randomly orienting both B850 rings in each trajectory. The uncertainty represents the 95% confidence interval. Full set of convergence parameters given in Table S6.

## S8. DIMER RATES: BRIGHT VS DARK

Recently, a model of LH2 excitation transport using Lindblad dynamics has suggested an important role for dark-state transport in close-packed LH2 complexes.[6] Fig S7a shows the distributions of dipole magnitude associated with each B850 monomer eigenstate over $10^4$ realizations of static disorder. We classify the first 3 eigenstates ($|\nu| \leq 2$) as bright states due to their large average dipole magnitude, while the remaining eigenstates ($|\nu| \geq 3$) are dark states.

The long-range transport predicted by the rate model described in the main text relies predominately on bright state inter-ring transport across all packing distances considered here. Fig S7b compares the rates of population transport with the full Hamiltonian (circles) and the Hamiltonian with inter-ring coupling via the dark-states removed (squares) at various

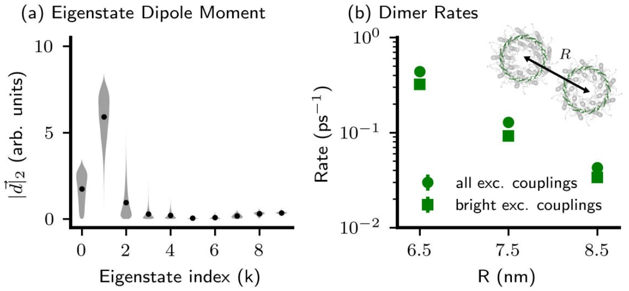


FIG. S7. B850 dimer. (a) The dipole moments of the eigenstates of an LH2 monomer over $10^4$ realizations of static disorder. (b) Transport rates for an LH2 dimer with an inter-ring separation of $R$ when all couplings are allowed (circles) and when inter-ring couplings involving dark states are forbidden (squares). In all cases, $\sigma = 160$ cm$^{-1}$ for site energy static disorder, and angular static disorder is given by randomly orienting both B850 rings in each trajectory. Full set of convergence parameters given in Table S6.

| Initial condition | Dark state transport | $\kappa_{dimer}$ (ps$^{-1}$) | Ratio |
|---|---|---|---|
| \|k\| = 1 | Allowed | 0.44±0.040 | 0.73 |
| | Forbidden | 0.32±0.023 | |
| From B800 | Allowed | 0.35±0.023 | 0.73 |
| | Forbidden | 0.25±0.013 | |

TABLE S3. The exponentially-fit exciton transfer rate $\kappa_{dimer}$ in a B850 dimer with inter-ring separation $R = 6.5$ nm with dark states both allowed and forbidden. The dark-state-allowed and dark-state-forbidden values of $\kappa_{dimer}$ (as well as the mean ratio between the two) are explored over two initial conditions. The uncertainty represents the 95% confidence interval. In all cases, $\sigma = 160$ cm$^{-1}$ for site energy static disorder. Full set of convergence parameters given in Table S6.

center-to-center dimer separations $R$. To remove dark-state couplings, we transformed the system Hamiltonian into the basis of B850 eigenstates and set all inter-ring couplings involving a dark state to 0. In all cases, we calculate the rate of transport ($\kappa_{dimer}$) by fitting the population dynamics starting from 600 fs, as described in the section S6. Removing dark state transport had a limited effect on the rate of transport across the inter-ring separations ($R$) studied here: the $\kappa_{dimer}$ is reduced to 73% of its original value when $R = 6.5$ nm. At center-to-center distances larger than 6.5 nm, the intra-monomer relaxation timescale is much faster than the inter-monomer transport rate, leading to an even smaller effect of removing dark states on the rate of transport for the $R = 7.5$ nm and $R = 8.5$ nm dimers. Thus, we find that the majority of transport takes place via bright state couplings, even in tightly-packed LH2 aggregates.

We find that the choice of initial condition does not change the role of dark states. Following the approach of Mattioni et al.,[6] we approximate the initial state of the donor B850 ring as the distribution expected when it acts as an excitation acceptor for the B800 ring. We account for the initial condition by creating an ensemble of initial states given by a distribution

| Parameter | Value (cm$^{-1}$) |
|---|---|
| $\gamma_{B850}$ | 20 |
| $\gamma_{B800}$ | 70 |
| $E$B800 | 12510 |

TABLE S4. Parameters introduced in Eq. (S7). Parameters are given by Mattioni et al. in Ref. 6.

over the monomer eigenstates $|\nu\rangle$ with weight $I_\nu$:

$$I_\nu = \frac{2\gamma_{B850}\Omega_\nu + \sum_{\nu'} W_{\nu'\nu}/2 + \gamma_{B800}}{(E_\nu - E_{B800})^2 + (2\gamma_{B850}\Omega_\nu + \sum_{\nu'} W_{\nu'\nu}/2 + \gamma_{B800})^2} \tag{S7}$$

with

$$\Omega_\nu = \sum_n \langle \nu|\hat{L}_n|\nu\rangle \tag{S8}$$

and

$$W_{\nu'\nu} = \sum_{\nu'} \frac{2\pi J(|\omega_{\nu'\nu}|)}{(e^{\nu_B T \omega_{\nu'\nu}} + 1)} \sum_n |\langle \nu'|\hat{L}_n|\nu\rangle|^2 \tag{S9}$$

where $\gamma_{B850}$ is the dephasing rate of a B850 ring Bchl, $\gamma_{B800}$ is the dephasing rate of a B800 ring Bchl, $E_{B800}$ is the average site energy of a B800 Bchl, $J(\omega)$ is the spectral density from main text eq. (9), $\hat{L}_n$ is the site-projection operator $|n\rangle\langle n|$, $E_\nu$ is the energy of $|\nu\rangle$, and $\omega_{\nu'\nu} = E_{\nu'} - E_\nu$.[6] Values of $\gamma_{B850}$, $\gamma_{B800}$, and $E_{B800}$ are given in Table S4. This distribution is averaged over $10^4$ realizations of site energy static disorder.

Table S3 compares the ensuing $\kappa_{dimer}$ in the case of allowed and forbidden dark state transport. While the change in initial state shifted the values of $\kappa_{dimer}$ in the case of allowed and forbidden dark state coupling in the $R = 6.5$ nm dimer, the ratio between these two rates was unchanged, with the removal of dark state couplings once more reducing $\kappa_{dimer}$ to 73% of its original value.

The dark-state transport mechanism found by Mattioni et al. arises from an exceptionally fast inter-ring transport rate predicted by their Lindblad calculations ($\kappa_{dimer} > 10$ ps$^{-1}$ at $R = 6.5$ nm). As a result, inter-ring transport occurs on a faster timescale than intra-ring exciton relaxation, supporting highly-populated dark states and exceptional dark state transport. Comparatively, in our formally-exact simulations, the rate of inter-ring transport is slower than intra-ring exciton relaxation even at $R = 6.5$ nm, leading to efficient relaxation into low-energy bright states and the dominant bright-state transport mechanism we observe.

## S9. DERIVING THE EXCITATION DIFFUSION LENGTH

We consider diffusive transport across a hexagonally-packed grid, where the excitation is originally localized on the central site ($P_0(0) = 1$). Each site is connected by the rate $\kappa$ to 6 symmetrically positioned nearest neighbors, giving rise to three independent directions. The number of steps from the origin ($\{a_n\}$) along each direction is given by an equation of motion,

$$\frac{dP_{a_n}(t)}{dt} = \kappa(P_{a_n-1}(t) + P_{a_n+1}(t) - 2P_{a_n}), \tag{S10}$$

which yields a 1-dimensional Gaussian distribution with expectation value $\langle a_n \rangle_t = 0$ for all $t$. The width of the distribution in units of steps, $\langle a_n^2 \rangle_t$, is given

$$\langle a_n^2 \rangle_t = \sum_{a_n=-\infty}^{\infty} a_n^2 P_{a_n}(t) \quad \text{(S11)}$$

which has a time-derivative

$$\frac{d}{dt}\langle a_n^2 \rangle_t = \sum_{a_n=-\infty}^{\infty} \kappa a_n^2 (P_{a_n-1}(t) + P_{a_n+1}(t) - 2P_{a_n}(t)) \quad \text{(S12)}$$

that can be solved by a shift of indexing and then explicit integration to give

$$\langle a_n^2 \rangle_t = 2\kappa t. \quad \text{(S13)}$$

Each independent step type is associated with displacement vector $\vec{q}_n =< x_n,\ y_n,\ z_n >$. We calculate the expectation of each mean-displacement term in Euclidean space:

$$\langle d^2 \rangle_t = \sum_{w=x,y,z} \sum_{n=1}^{3} \langle a_n^2 \rangle_t w_n^2 = \sum_{w=x,y,z} \sum_{n=1}^{3} 2\kappa t w_n^2 \quad \text{(S14)}$$

where the displacement vectors $\vec{q}_1 = \pm < R, 0, 0 >$, $\vec{q}_2 = \pm < \frac{R}{2}, \frac{\sqrt{3}R}{2}, 0 >$, and $\vec{q}_3 = \pm < -\frac{R}{2}, \frac{\sqrt{3}R}{2}, 0 >$ are defined as functions of the packing distance $R$. Thus, $\langle d^2 \rangle_t = 6\kappa R^2 t$. The diffusion length $L_d$ is defined by

$$L_d = \sqrt{\langle d^2 \rangle}_\tau = R\sqrt{6\kappa\tau} \quad \text{(S15)}$$

where $\tau$ is the excitation lifetime.

We note this derivation holds for any packing described by a regular polygon with an even number of vertices, and generalizes to

$$\langle d^2 \rangle_t = N\kappa R^2 t \text{ and } L_d = R\sqrt{N\kappa\tau} \quad \text{(S16)}$$

where $N$ is the number of vertices of the polygon (i.e., the number of nearest neighbors).

## REFERENCES


[1] G. D. Scholes and G. R. Fleming, "On the mechanism of light harvesting in photosynthetic purple bacteria: B800 to b850 energy transfer," J. Phys. Chem. B **104**, 1854–1868 (2000).

[2] C. Smyth, D. G. Oblinsky, and G. D. Scholes, "B800–B850 coherence correlates with energy transfer rates in the LH2 complex of photosynthetic purple bacteria," Phys. Chem. Chem. Phys. **17**, 30805–30816 (2015).

[3] L. Varvelo, J. K. Lynd, and D. I. G. Bennett, "Eformally exact simulations of mesoscale exciton dynamics in molecular materials," Chemical Science **12**, 9704–9711 (2021).

[4] D. B. Percival, "Exact simulation of complex-valued gaussian stationary processes via circulant embedding," Signal Process. **86**, 1470–1476 (2006).

[5] M. Escalante, A. Lenferink, Y. Zhao, N. Tas, J. Huskens, C. N. Hunter, V. Subramaniam, and C. Otto, "Long-range energy propagation in nanometer arrays of light harvesting antenna complexes," Nano Lett. **10**, 1450–1457 (2010).

[6] A. Mattioni, F. Caycedo-Soler, S. F. Huelga, and M. B. Plenio, "Design Principles for Long-Range Energy Transfer at Room Temperature," Physical Review X **11**, 041003 (2021).

| Simulation | $k_{max}$ | $k_{Mats}$ | $dt$ (fs) | $\delta_A$ | $\delta_S$ | $u_t$ (fs) | $N_{traj}$ |
|---|---|---|---|---|---|---|---|
| Figs. S6/S7 - 6.5 nm dark states allowed | 10 | 5 | 2.0 | 0.005 | 0 | 20 | $10^4$ |
| Fig. S7 - 6.5 nm dark states forbidden | 10 | 2 | 1.0 | 0.0015 | 0 | 20 | $10^4$ |
| Fig. S7 - 7.5 nm dark states allowed | 10 | 10 | 1.0 | 0.0015 | 0 | 8.0 | $10^4$ |
| Fig. S7 - 7.5 nm dark states forbidden | 50 | 20 | 0.5 | 0.0005 | 0 | 4.0 | $10^4$ |
| Fig. S7 - 8.5 nm dark states allowed | 50 | 20 | 0.5 | 0.001 | 0 | 20 | $10^4$ |
| Fig. S7 - 8.5 nm dark states forbidden | 50 | 20 | 0.125 | 0.0005 | 0 | 10 | $10^4$ |
| Table S3 - Initial condition from B800 | 10 | 5 | 1.0 | 0.0015 | 0 | 10 | $10^4$ |
| Fig. S1a - hierarchy depth | varies | 2 | 2.0 | 0.0015 | 0 | 2.0 | $\in [999, 1000]$ |
| Fig. S1b - hierarchy adaptivity | 50 | 2 | 2.0 | varies | 0 | 2.0 | $10^3$ |
| Fig. S1c - timestep | 20 | 2 | varies | 0.0015 | 0 | 2.0 | $\in [999, 1000]$ |
| Fig. S1d - update time | 10 | 2 | 2.0 | 0.0015 | 0 | varies | $10^3$ |
| Fig. S1e - Matsubara modes | 20 | varies | 0.5 | 0.0015 | 0 | 2.0 | $10^3$ |
| Fig. S1f - state adaptivity | 10 | 2 | 2.0 | 0.0015 | varies | 20 | $10^3$ |
| Fig. S2a - hierarchy adaptivity | 50 | 20 | 0.25 | varies | 0 | 2.0 | $\in [999, 1000]$ |
| Fig. S2b - timestep | 10 | 1 | varies | 0.005 | 0 | $\min(2.0, dt)$ | $10^4$ |
| Fig. S2c - update time | 10 | 2 | 2.0 | 0.0015 | 0 | varies | $10^3$ |
| Fig. S2d - Matsubara modes | 10 | varies | 0.25 | 0.005 | 0 | 2.0 | $10^3$ |
| Fig. S3a - hierarchy adaptivity | 50 | 20 | 0.25 | varies | 0 | 2.0 | $10^3$ |
| Fig. S3b - timestep | 50 | 20 | varies | 0.0015 | 0 | 16 | $\in [995, 1000]$ |
| Fig. S3c - update time | 50 | 20 | 0.25 | 0.0015 | 0 | varies | $\in [999, 1000]$ |
| Fig. S4a - hierarchy adaptivity | 50 | 20 | 0.25 | varies | 0 | 2.0 | $\in [998, 1000]$ |
| Fig. S4b - update time | 50 | 20 | 0.5 | 0.001 | 0 | varies | $\in [998, 1000]$ |
| Fig. S5a - hierarchy adaptivity (heptamer) | 10 | 5 | 2.0 | varies | 0 | 8.0 | $\in [995, 1000]$ |
| Fig. S5b - Matsubara modes (heptamer) | 10 | varies | 0.5 | 0.005 | 0 | 20 | $10^3$ |
| Fig. S5c - timestep (heptamer) | 10 | 5 | varies | 0.005 | 0 | 20 | $10^3$ |
| Fig. S5d - update time | 10 | 5 | 2.0 | 0.005 | 0.005 | varies | $10^3$ |
| Fig. S5e - state adaptivity (heptamer) | 10 | 5 | 2.0 | 0.005 | varies | 8.0 | $\in [999, 1000]$ |
| Fig. S5f - state adaptivity (37-mer) | 10 | 5 | 2.0 | 0.005 | varies | 20 | $\in [983, 1000]$ |
| Table S2 - all cases | 10 | 5 | 2.0 | 0.005 | 0 | 20 | $10^4$ |

TABLE S5. The convergence parameters of all simulations recorded in the Supporting Information.

| Simulation | $k_{max}$ | $k_{Mats}$ | $dt$ (fs) | $\delta_A$ | $\delta_S$ | $u_t$ (fs) | $N_{traj}$ |
|---|---|---|---|---|---|---|---|
| Fig. 1 | 10 | 2 | 1.0 | 0.0015 | 0 | 20 | $10^4$ |
| Fig. 2 | 10 | 5 | 2.0 | 0.005 | 0.0035 | 20 | 992 |
| Fig. 3/Table 1 - 6.5 nm | 10 | 5 | 2.0 | 0.005 | 0 | 20 | $10^4$ |
| Fig. 3/Table 1 - 7.5 nm | 10 | 10 | 1.0 | 0.0015 | 0 | 8.0 | $10^4$ |
| Fig. 3/Table 1 - 8.5 nm | 50 | 20 | 0.5 | 0.001 | 0 | 20 | $10^4$ |

TABLE S6. The convergence parameters of all simulations recorded in the main text.
